# Supplementary material for: FOCUS: Flexible Optimizable Counterfactual Explanations for Tree Ensembles
Source: arXiv:1911.12199 source file (2021-12-17)
Supplement: Supplementary file 1 [file appendix.tex]

%!TEX root = ../focus_rai_kdd_4pg.tex

\appendix

\pagebreak

\section{Models DACE Can't Run On}
\label{section:dace-failures}
We were unable to run DACE on the following settings because the problem size is too large when using the free Python API of CPLEX:
\begin{itemize}[leftmargin=*]
	\item Wine Quality AB (100 trees, max depth 4)
	\item Wine Quality RF (500 trees, max depth 4)
	\item HELOC RF (500 trees, max depth 4)
	\item HELOC AB (100 trees, max depth 8)
	\item COMPAS RF (500 trees, max depth 4)
	\item Shopping RF (500 trees, max depth 8).
\end{itemize}
We note that these are not unreasonable model sizes, and that unlike DACE, \OurMethod{} can be applied to all \numprint{12} models (see Table~\ref{table:distances}).

\section{Evaluation Metrics}
\label{section:metrics}
Here we show exact calculations for mean distance ($d_\mathit{mean}$) and mean relative distance ($d_\mathit{Rmean}$). 
Let $X$ be the set of $N$ original instances and $\bar{X}$ be the corresponding set of $N$ generated counterfactual examples.
The mean distance is defined as:
\begin{equation}
\label{eq:mean-dist}
d_\mathit{mean}(X, \bar{X}) = \frac{1}{N}\sum_{n=1}^{N}d(x^{(n)}, \bar{x}^{(n)}).
\end{equation}

Let $\bar{X}$ be the set of counterfactual examples produced by \OurMethod{} and let $\bar{X}'$ be the set of counterfactual examples produced by a baseline. 
Then the mean relative distance is defined as:
\begin{equation}
\label{eq:mean-rel-dist}
d_\mathit{Rmean}(\bar{X}, \bar{X}') = \frac{1}{N}\sum_{n=1}^{N} \frac{d(x^{(n)}, \bar{x}^{(n)})}{d(x^{(n)}, {\bar{x}}^{'(n)})}.
\end{equation}

\section{Fidelity of Approximations}
Fidelity is commonly used to evaluate XAI methods that are based on approximations of a given model: it is a measure of the agreement between the original model $\mathcal{M}$ and its approximation $\widetilde{\mathcal{M}}$: 
\begin{align}
\begin{split}
%\mbox{}\hspace*{-1.5mm}
\textit{fid}(\widetilde{\mathcal{M}}, X) \!=\! 
\frac{1}{N} \sum_{n=1}^N
\mathbbm{1}\left[
y_{x^{(n)}}
\!=\! \arg\max_{y'} \widetilde{\mathcal{M}}(y' | x^{(n)})
\right],
%\hspace*{-1mm}\mbox{}
\end{split}
\end{align}
where $y_x = \arg\max_{y} \mathcal{M}(y \mid x)$. 
In our case, the purpose of the approximations is not to replace the original models, but rather to construct differentiable versions of the models so we can generate counterfactual examples through gradient-based optimization. 
Examining the fidelity is meant as a \emph{sanity check} -- to ensure our approximations are reasonably representative of the original model.

Table~\ref{table:fidelity} shows the fidelity of the model approximations used in our experiments: a value of \numprint{1} indicates perfect alignment between $\mathcal{M}$ and $\widetilde{\mathcal{M}}$. 
We see that the alignment is at least \numprint{0.7}, which indicates that \OurMethod{} approximations are indeed reasonable representations of the original model -- both in terms of their inner workings (i.e., same tree structure, same features, same splitting thresholds but ``softer'' versions) as well as their predictions.

\begin{table}
\centering
\caption{Fidelity of FOCUS approximations used in Experiments \numprint{1} and \numprint{2}: --- denotes models we were unable to run DACE on.
The parameters $\sigma$ and $\tau$ are chosen per setting based on which values produce the best counterfactual examples.
As a result, different approximations of the same model are used when optimizing for different distance functions, but in some cases (e.g., \textit{Wine Quality} DT), the approximations are the same regardless of the distance function.}

\begin{tabular}{lcrrrr}
\toprule
\textbf{Dataset}              & \textbf{Model} & \multicolumn{1}{c}{\textbf{Euclid.}} & \multicolumn{1}{c}{\textbf{Cosine}} & \multicolumn{1}{c}{\textbf{Man.}} & \multicolumn{1}{c}{\textbf{Mah.}} \\
\midrule
\textit{Wine} & DT             & 0.836     & 0.836  & 0.836    &	0.900\\

    \textit{Quality}                          & RF             		& 0.940     & 0.940  & 0.940  &  --- \\
                              & AB       			& 0.926     & 0.926  & 0.926   &  --- \\
\midrule
\multirow{3}{*}{\textit{HELOC}}        & DT             & 0.836     & 0.836  & 0.836  &   0.930 \\
                              & RF             		& 0.954     & 0.887  & 0.887   &  --- \\
                              & AB       			& 0.936     & 0.744  & 0.905    & --- \\
\midrule
\multirow{3}{*}{\textit{COMPAS}} & DT    	& 0.844     & 0.894  & 0.807   &  0.807 \\
						& RF 	& 0.742     & 0.809  & 0.700   &  --- \\
						& AB		& 0.922     & 0.922  & 0.814   &  0.814 \\
						
\midrule
\multirow{3}{*}{\textit{Shopping}} & DT    	& 0.902     & 0.906  & 0.902  &   0.902 \\
						& RF 	& 0.810     & 0.780  & 0.871   &  --- \\
						& AB		& 0.919     & 0.919  & 0.919	& 0.919	\\
\bottomrule     
\end{tabular}
%}
\label{table:fidelity}
\end{table}

\if0
\section{Related Work}
\label{section:relatedwork}

\subsection{Algorithmic Recourse}
%\todo{Algorithmic recourse: \citet{ustun_actionable_2019}, \citet{joshi_towards_2019}, \citet{karimi_recourse_2020}, \citet{karimi_imperfect_causal_2020}}
%\todo{Highlight how unrealistic the causal ones are, and how the developers shouldn't be the arbiters of actionability. The point of counterfactual explanations (as noted by Wachter is not only to create change, but also to understand what the model gives value to. Also recourse can only be guaranteed with linear models.}

Algorithmic recourse is a line of research that is closely related to counterfactual explanations, except that these methods include the additional restriction that the resulting explanation must be \emph{actionable} \citep{ustun_actionable_2019, joshi_towards_2019, karimi_recourse_2020, karimi_imperfect_causal_2020}. 
This is done by selecting a subset of the features to which perturbations can be applied in order to avoid explanations that suggest impossible or unrealistic changes to the feature values (i.e., change \textit{age} from \numprint{25} $\to$ \numprint{50} or change \textit{marital\_status} from $\mathrm{MARRIED}$ $\to$ UNMARRIED). 
Although this work has produced impressive theoretical results, it is unclear how realistic they are in practice, especially for complex ML models such as tree ensembles. 
Existing algorithmic recourse methods cannot solve our task because they 
\begin{enumerate*}[label=(\roman*)]
	\item are either restricted to solely linear \citep{ustun_actionable_2019} or  differentiable \citep{joshi_towards_2019} models, or
	\item  require access to causal information \citep{karimi_recourse_2020, karimi_imperfect_causal_2020}, which is rarely available in real world settings. 
\end{enumerate*}
%\citet{ustun_actionable_2019} originally formulate the task of algorithmic recourse and provide some theoretical guarantees in the context of linear classification, but the method is not applicable to tree-based models. 
% \citet{joshi_towards_2019} propose a model based on modeling the data manifold, but this is only applicable to differentiable models. 
%The methods of \cite{karimi_recourse_2020} and \cite{karimi_imperfect_causal_2020} both require access to the underlying causal graph, which is rarely available in practice and very difficult to generate from data alone. 
%\cite{karimi_recourse_2020} also requires access to the underlying structural causal model. 

Another shortcoming of algorithmic recourse methods is that they require that the actionable subset of features is determined \emph{in advance}, which can often mean that developers are put in the position of determining what is actionable. 
Although this is obvious for some features (i.e., age), actionability is not necessarily a binary condition, and what is actionable for one person may not be actionable for another \citep{barocas_hidden_2019}. 
Moreover, if we restrict the perturbations to only act on actionable features, we lose sight of any non-actionable features that the model deems important -- although it is unrealistic to ask someone to change their age, it is still important to know that the model's decisions depend on age. 
This also allows the user to contest the use of such a feature in determining their outcome. 

Unlike algorithmic recourse methods, our work does not necessarily aim to provide the user with the definitive set of feature value changes they need for a different outcome. 
In contrast, we provide a counterfactual ``menu of options'' \citep{barocas_hidden_2019} that can be customized based on the chosen distance function. 
Although counterfactual explanations may be less actionable than algorithmic recourse methods, they provide a more complete picture of what is important to the model and allow the end-user to decide what is (not) actionable for themselves. 
Counterfactual explanations are meant to serve as a starting point for recourse: we argue that the task of recourse should not be solved from a purely algorithmic perspective, but rather as part of a human-in-the-loop process. 
Counterfactual explanations therefore provide the user with a more complete notion of potential feature value changes in comparison to existing algorithmic recourse methods, and serve as the algorithmic component of achieving recourse.

\subsection{Model-specific Counterfactual Examples}
We propose a model-specific approach for generating counterfactual examples. %\HHcomment{Should the section start with this? then enumerate what others do? sounds like you explain your work all over again}
Previous model-specific work has either been done through optimization \citep{wachter_counterfactual_2017, grath_interpretable_2018, dhurandhar_explanations_2018}, mixed integer programming \citep{russell_efficient_2019, kanamori_dace_2020}, or heuristic search \citep{tolomei_interpretable_2017}. 
Some of this work is applicable to linear models or neural networks \citep{wachter_counterfactual_2017, grath_interpretable_2018, dhurandhar_explanations_2018, russell_efficient_2019}, while other work can be applied to tree-ensembles \citep{tolomei_interpretable_2017, kanamori_dace_2020}. 

Our work is the first model-specific approach for generating counterfactual examples for tree ensembles through gradient-based optimization. 
We compare our method against existing approaches for tree-ensembles \citep{tolomei_interpretable_2017, kanamori_dace_2020}, and refer the reader to Appendix~\ref{section:baselines} for a more detailed overview of these methods.

\subsection{Adversarial Examples}
Adversarial examples are a type of counterfactual example with the additional constraint that the minimal perturbation results in an alternative prediction that is \emph{incorrect}. 
There are a variety of methods for generating adversarial examples \cite{goodfellow_explaining_2015,szegedy_intriguing_2014,su_one_2019,brown_adversarial_2018}; a more complete overview can be found in \cite{biggio_wild_2018}. 
%Adversarial examples are minimal perturbations to the input such that the prediction is \emph{incorrect}. 
%This is closely related to counterfactual examples since in both cases, we are trying to generate examples with an alternative prediction. 

%In the case of adversarial examples, we have the additional criteria that the original instance should have the correct prediction, whereas this is not necessarily the case for counterfactual examples. 

The main difference between adversarial examples and counterfactual examples is in the intent: adversarial examples are meant to \emph{fool} the model, whereas counterfactual examples are meant to \emph{explain} the model.\footnote{However, it also is possible to use counterfactual examples for fooling, and adversarial examples for explaining, as they are closely related.}
Another difference is that adversarial examples are typically studied in the context of image classification, whereas counterfactual examples are usually studied in the context of tabular or textual data. 
Perturbations to pixels in an image often result in changes that are undetectable to the human eye, whereas perturbations to feature values or the presence/absence of terms in a sentence are meant to be detectable, since this is what the explanation is created from. 

\subsection{Local Explanations}

Our work is part of a broader family of local explanation methods that use model approximation in the pipeline of explaining individual predictions. 
Other common approaches to local explanations involve approximating the original model locally with an inherently interpretable explanator (i.e., linear regression, shallow decision tree) to derive feature importances or decision rules \citep{guidotti_local_2018, ribeiro-2016-should}. 
A shortcoming of these approaches is that the approximation is not necessarily guaranteed to mimic the original model, since it is typically a simpler version which is only valid locally. 
%\HHcomment{additional limitations (to add?): instability of explanations based on sampling,  ignoring dependency between features, neighborhood definition around instance to explain}

This work is similar to ours in that it uses model approximations to explain individual predictions, but it differs from ours because:
\begin{enumerate*}[label=(\roman*)]
\item the approximations are local -- they only hold around the point in question, and
\item our objective is not to simplify the model, but rather to produce a differentiable version in order to leverage gradient-based optimization techniques. 
\end{enumerate*}
In other words, previous methods generate local explanations via local approximations, while our method generates local explanations via global approximations. 

\subsection{Differentiable Trees}
Part of our contribution involves constructing differentiable versions of tree ensembles by replacing each splitting threshold with a sigmoid function. 
This can be seen as using a (small) neural network to obtain a smooth approximation of each tree. 
%Other differentiable versions of trees include neural decision trees \citep{balestriero_neural_2017, yang_deep_2018} and soft decision trees~\citep{hinton_distilling_2014}. 
Neural decision trees \citep{balestriero_neural_2017, yang_deep_2018} are also differentiable versions of trees, which use a full neural network instead of a simple sigmoid. 
However, these do not optimize for approximating an already trained model. Therefore, unlike our method, they are not an obvious choice for finding counterfactual examples for an existing model. 
Soft decision trees~\citep{hinton_distilling_2014} are another example of differentiable trees, which instead approximate a neural network with a decision tree. 
This can be seen as the inverse of our task. 

%\todo{Model distillation \citet{tan_distill-and-compare_2018}}
\fi
